# Supplementary material for: PixLens: A Novel Framework for Disentangled Evaluation in Diffusion-Based Image Editing with Object Detection + SAM
Source: arXiv:2410.05710 source file (2024-10-08)
Supplement: Supplementary file 1 [file disentanglement_confusion.tex]

\documentclass[tikz]{standalone}
\usepackage{ifthen}
\usetikzlibrary{matrix,calc}

\begin{document}

%The matrix in numbers
%Horizontal target class
%Vertical output class
\def\myConfMat{{
{100.91,  0.09,  0.00,   0.00},  %row 1
{   0.00,0.93, 0.07,  0.00},  %row 2
{   0.00,  0.14,0.86, 0.00},  %row 3
{   0.00, 0.09,  0.00,0.91},  %row 4
}}

\def\classNames{{"Color","Patttern","Style","Texture"}} %class names. Adapt at will

\def\numClasses{4} %number of classes. Could be automatic, but you can change it for tests.

\def\myScale{1.5} % 1.5 is a good scale. Values under 1 may need smaller fonts!
\begin{tikzpicture}[
    scale = \myScale,
    %font={\scriptsize}, %for smaller scales, even \tiny may be useful
    ]

\tikzset{vertical label/.style={rotate=90,anchor=east}}   % usable styles for below
\tikzset{diagonal label/.style={rotate=45,anchor=north east}}

\foreach \y in {1,...,\numClasses} %loop vertical starting on top
{
    % Add class name on the left
    \node [anchor=east] at (0.4,-\y) {\pgfmathparse{\classNames[\y-1]}\pgfmathresult}; 
    
    \foreach \x in {1,...,\numClasses}  %loop horizontal starting on left
    {
%---- Start of automatic calculation of totSamples for the column ------------   
    \def\totSamples{0}
    \foreach \ll in {1,...,\numClasses}
    {
        \pgfmathparse{\myConfMat[\ll-1][\x-1]}   %fetch next element
        \xdef\totSamples{\totSamples+\pgfmathresult} %accumulate it with previous sum
        %must use \xdef fro global effect otherwise lost in foreach loop!
    }
    \pgfmathparse{\totSamples} \xdef\totSamples{\pgfmathresult}  % put the final sum in variable
%---- End of automatic calculation of totSamples ----------------
    
    \begin{scope}[shift={(\x,-\y)}]
        \def\mVal{\myConfMat[\y-1][\x-1]} % The value at index y,x (-1 because of zero indexing)
        \pgfmathtruncatemacro{\r}{\mVal}   %
        \pgfmathtruncatemacro{\p}{round(\r/\totSamples*100)}
        \coordinate (C) at (0,0);
        \ifthenelse{\p<50}{\def\txtcol{black}}{\def\txtcol{white}} %decide text color for contrast
        \node[
            draw,                 %draw lines
            text=\txtcol,         %text color (automatic for better contrast)
            align=center,         %align text inside cells (also for wrapping)
            fill=black!\p,        %intensity of fill (can change base color)
            minimum size=\myScale*10mm,    %cell size to fit the scale and integer dimensions (in cm)
            inner sep=0,          %remove all inner gaps to save space in small scales
            ] (C) {\r\\\p\%};     %text to put in cell (adapt at will)
        %Now if last vertical class add its label at the bottom
        \ifthenelse{\y=\numClasses}{
        \node [] at ($(C)-(0,0.75)$) % can use vertical or diagonal label as option
        {\pgfmathparse{\classNames[\x-1]}\pgfmathresult};}{}
    \end{scope}
    }
}
%Now add x and y labels on suitable coordinates
\coordinate (yaxis) at (-0.9,0.5-\numClasses/2);  %must adapt if class labels are wider!
\coordinate (xaxis) at (0.5+\numClasses/2, -\numClasses-1.25); %id. for non horizontal labels!
\node [vertical label] at (yaxis) {Actual Class};
\node []               at (xaxis) {Predicted Class};
\end{tikzpicture}

\end{document}
